# Supplementary material for: Attitude Control of Spacecraft for Autonomous Attenuation of Unknown Periodic Disturbance Torque
Source: arXiv:2505.00355 source file (2025-05-01)
Supplement: Supplementary file 1 [file Appendix.tex]

\section{Appendix}
Equation~\ref{eq:New dynamics and kinematics} can be rewritten as follows.
\begin{equation}
    \dot{\bm{x}}(t) = \bm{f}[\bm{x}(t)]+\bm{B}\bm{u}^{\mathrm{rc}}(t)+\bm{B}\bm{T}_{\mathrm{ext}}(t)
    \label{eq:eq_new}
\end{equation}
where
\begin{equation}
    \bm{x}(t) = 
    \begin{bmatrix}
        \delta \bm{q}(t)\\
        \delta \bm{\omega}(t)
    \end{bmatrix}
\end{equation}
\begin{equation}
    \bm{f}[\bm{x}(t)]=
    \begin{bmatrix}
        \frac{1}{2}[\delta q_{4}\bm{I}_3+\delta\bm{q}^{\times}]\delta\bm{\omega}(t)\\
        \delta\bm{\omega}(t)^{\times}\bm{R}[\delta\bar{q}(t)]\bm{\omega}_d(t)
    \end{bmatrix}
\end{equation}
\begin{equation}
    \bm{B} = 
    \begin{bmatrix}
        0_{3 \times 3}\\
        \bm{J}^{-1}
    \end{bmatrix}
\end{equation}
Integrating Eq.~\ref{eq:eq_new} results in
\begin{equation}
    \bm{x}(t+\Delta)=\bm{x}(t)+\int_{t}^{t+\Delta}\left\{\bm{f}[\bm{x}(\tau)]+\bm{B}\bm{u}^{\mathrm{rc}}(\tau)+\bm{B}\bm{T}_{\mathrm{ext}}(\tau)\right\}d\tau
    \label{eq:Integrating}
\end{equation}
Using the anticipatory RC updating law in Eq.~\ref{eq:RC scheme} yields the following input error equation. 
\begin{equation}
    \bm{u}^{rc}(t) = \bm{u}^{rc}(t-T)-\bm{L}(\cdot)\bm{x}(t-T+\Delta)
    \label{eq:RC new}
\end{equation}
where
\begin{equation}
    \bm{L}(\cdot) = [k^{rc}_p\bm{J}\quad k^{rc}_d\bm{J}]
\end{equation}
Substituting Eq.~\ref{eq:Integrating} into Eq.~\ref{eq:RC new} yields
\begin{equation}
    \begin{aligned}
        \bm{u}^{rc}(t)&=\bm{u}^{rc}(t-T)-\bm{L}(\cdot)\bm{B}\int_{t}^{t+\Delta}\bm{u}^{rc}(\tau-T)d\tau-\bm{L}(\cdot)\bm{x}(t-T)\\&-\bm{L}(\cdot)\int_{t}^{t+\Delta}\bm{f}[\bm{x}(\tau-T)]d\tau-\bm{L}(\cdot)\bm{B}\int_{t}^{t+\Delta}\bm{T}_{\mathrm{ext}}(\tau-T)d\tau\ \\
        &=[\mathrm{I}-\Delta\bm{L}(\cdot)\bm{B}]\bm{u}^{rc}(t-T)-\bm{L}(\cdot)\bm{x}(t-T)-\bm{L}(\cdot)\int_{t}^{t+\Delta}\bm{f}[\bm{x}(\tau-T)]d\tau\\
        &-\bm{L}(\cdot)\bm{B}\int_{t}^{t+\Delta}\bm{T}_{\mathrm{ext}}(\tau-T)d\tau-\bm{L}(\cdot)\bm{B}\int_{t}^{t+\Delta}\Delta\dot{\bm{u}}^{rc}(\tau-T)d\tau\\
        &=(1-\Delta\cdot k^{rc}_d)\bm{u}^{rc}(t-T)-\bm{L}(\cdot)\bm{x}(t-T)-\bm{L}(\cdot)\int_{t}^{t+\Delta}\bm{f}[\bm{x}(\tau-T)]d\tau\\
        &-\bm{L}(\cdot)\bm{B}\int_{t}^{t+\Delta}\bm{T}_{\mathrm{ext}}(\tau-T)d\tau-\bm{L}(\cdot)\bm{B}\int_{t}^{t+\Delta}\Delta\dot{\bm{u}}^{rc}(\tau-T)d\tau\\
    \end{aligned}
\end{equation}
Taking norms on both sides,
\begin{equation}
    \begin{aligned}
    ||\bm{u}^{rc}(t)||&\leq\rho||\bm{u}^{rc}(t-T)||+b_L||\bm{x}(t-T)||+b_Lc_f\int_{t}^{t+\Delta}||\bm{x}(\tau-T)||d\tau+b_Lb_Bb_T\Delta+O(\Delta^2)\\
    &\leq \rho||\bm{u}^{rc}(t-T)||+(b_L+\Delta b_Lc_f)||\bm{x}(t-T)||+b_Lb_Bb_T\Delta+O(\Delta^2)
    \label{eq:norm}
    \end{aligned}
\end{equation}
where $b_L$ and $b_B$ are the norm bounds for $\bm{L}(\cdot)$ and $\bm{B}$, respectively. The following uniformly global Lipschitz condition about the function $\bm{f}(\bm{x}(t))$ is used in Eq.~\ref{eq:norm}.
\begin{equation}
    ||\bm{f}[\bm{x}(t)]||\leq c_f||\bm{x}(t)||
\end{equation}
Writing the integral expression for $\bm{x}(t)$ and taking norms is described as follows.
\begin{equation}
    \begin{aligned}
    ||\bm{x}(t)||&=\left\|\bm{x}(0)+\int^t_0\left\{\bm{f}[\bm{x}(\tau)]+\bm{B}\bm{u}^{rc}(\tau)+\bm{B}\bm{T}_{\mathrm{ext}}(\tau)\right\}d\tau\right\|\\
    &\leq ||\bm{x}(0)||+\int^t_0\left\{c_f||\bm{x}(\tau)||+b_B||\bm{u}^{rc}(\tau)||+b_Bb_T\right\}d\tau
    \end{aligned}
    \label{eq:intnorm_t}
\end{equation}
$\bm{x}(t)$ before one cycle can be expressed as follows.
\begin{equation}
    ||\bm{x}(t-T)||\leq ||\bm{x}(0)||+\int^t_0\left\{c_f||\bm{x}(\tau-T)||+b_B||\bm{u}^{rc}(\tau-T)||+b_Bb_T\right\}d\tau
    \label{eq:intnorm}
\end{equation}
Then, using Bellman–Gronwall inequality in Eqs.~\ref{eq:intnorm_t} and~\ref{eq:intnorm}, it is expressed as follows.
\begin{equation}
    ||\bm{x}(t)||\leq ||\bm{x}(0)||e^{c_ft}+\int^t_0e^{c_f(t-\tau)}\left\{b_B||\bm{u}^{rc}(\tau)||+b_Bb_T\right\}d\tau
    \label{eq:Gronwall_0}
\end{equation}
\begin{equation}
    ||\bm{x}(t-T)||\leq ||\bm{x}(0)||e^{c_ft}+\int^t_0e^{c_f(t-\tau)}\left\{b_B||\bm{u}^{rc}(\tau-T)||+b_Bb_T\right\}d\tau
    \label{eq:Gronwall}
\end{equation}
Combining Eqs.~\ref{eq:norm} and \ref{eq:Gronwall} yields
\begin{equation}
    \begin{aligned}
    ||\bm{u}^{rc}(t)||&\leq\rho||\bm{u}^{rc}(t-T)||+(b_L+\Delta b_Lc_f)\left\{||\bm{x}(0)||e^{c_ft}+\int^t_0e^{c_f(t-\tau)}\left[b_B||\bm{u}^{rc}(\tau-T)+b_Bb_T\right]d\tau\right\}\\
    &+b_Lb_Bb_T+O(\Delta^2)\\
    &\leq \rho||\bm{u}^{rc}(t-T)||+(b_L+\Delta b_Lc_f)b_B\int^t_0e^{c_f(t-\tau)}||\bm{u}^{rc}(t-\tau)d\tau+(b_L+\Delta b_Lc_f)||\bm{x}(0)e^{c_ft}\\
    &+(b_L+\Delta b_Lc_f)b_Bb_T\int^t_0e^{c_f(t-\tau)}+b_Lb_Bb_T\Delta+O(\Delta^2)
    \end{aligned}
    \label{eq:combine}
\end{equation}
Multiplying Eq.~\ref{eq:combine} by $e^{-\lambda t}$, defining $k \triangleq \mathrm{max}\left\{(b_L+\Delta b_Lc_f)b_B, c_f\right\}$, and assuming $ \lambda > k$ yields
\begin{equation}
    \begin{aligned}
    e^{-\lambda t}||\bm{u}^{rc}(t)||&\leq e^{-\lambda t}\rho||\bm{u}^{rc}(t-T)||+k\int^t_0e^{\lambda t}||\bm{u}^{rc}(\tau-T)||e^{(k-\lambda)(t-\tau)}d\tau+(b_L+\Delta b_Lc_f)||\bm{x}(0)||e^{(c_f-\lambda)t}\\
    &+(b_L+\Delta b_Lc_f)b_Bb_T\int^t_0e^{-\lambda t}e^{(c_f-\lambda)(t-\tau)}d\tau+b_Lb_Bb_T\Delta e^{-\lambda t}+O(\Delta^2)
    \end{aligned}
\end{equation}
Noticing that the integrals are strictly increasing and that for a constant $||k||_{\lambda}=k$ results in
\begin{equation}
    \begin{aligned}
    ||\bm{u}^{rc}(t)||_{\lambda}&\leq\left[\rho+\frac{k}{\lambda-k}(1-e^{(k-\lambda)T'}) \right]||\bm{u}^{rc}(t-T)||_{\lambda}+(b_L+\Delta b_Lc_f)||\bm{x}(0)||\\
    &+\frac{(b_L+\Delta b_Lc_f)b_Bb_T}{\lambda-c_f}(1-e^{(c_f-\lambda)T'})+b_Lb_Bb_T\Delta+O(\Delta^2)
    \end{aligned}
    \label{eq:u_norm}
\end{equation}
where $||\cdot||_\lambda$ denotes the $\lambda$ norm of a vector. \\
Define 
\begin{equation}
    \begin{aligned}
    \bar{\rho} &= \left[\rho+\frac{k}{\lambda-k}(1-e^{(k-\lambda)T'})\right]\\
    k_2 &= ((b_L+\Delta b_Lc_f)\\
    k_3 &= b_Lb_B\Delta+\frac{(b_L+\Delta b_Lc_f)b_Bb_T}{\lambda-c_f}(1-e^{(c_f-\lambda)T'})
    \end{aligned}
\end{equation}
Equation~\ref{eq:u_norm} can be rewritten as follows.
\begin{equation}
    ||\bm{u}^{rc}(t)||_{\lambda}\leq\bar{\rho}||\bm{u}^{rc}(t-T)||_{\lambda}+k_2||\bm{x}(0)||+k_3b_T+O(\Delta^2)
\end{equation}
\begin{equation}
    ||\bm{u}^{rc}(t)||_{\lambda}\leq\bar{\rho}||\bm{u}^{rc}(t-T)||_{\lambda}+\epsilon
\end{equation}
where
\begin{equation}
    \epsilon = k_2||\bm{x}(0)||+k_3b_T+O(\Delta^2)
    \label{eq:eps}
\end{equation}
Since $\rho < 1$, $\lambda > k$ can be found such that $\rho < 1$.
Thus $u^{rc}(t)$ converges to a neighborhood of zero of radius $\epsilon/(1-\bar{\rho})$ with respect to the $\lambda-$norm.
\begin{equation}
    \lim_{t\rightarrow\infty}\sup||\bm{u}^{rc}(t)||_{\lambda}\leq\frac{1}{1-\bar{\rho}}\epsilon
\end{equation}
In Eq.~\ref{eq:Gronwall_0}, a similar manipulation is applied. 
Multiplying Eq.~\ref{eq:Gronwall_0} by $e^{-\lambda t}$, defining $k \triangleq \mathrm{max}\left\{(b_L+\Delta b_Lc_f)b_B, c_f\right\}$, and assuming $ \lambda > k$ yields
\begin{align}
    e^{-\lambda t}||\bm{x}(t)||&\leq||\bm{x}(0)||e^{(c_f-\lambda)t}+\int^t_0e^{(c_f-\lambda)(t-\tau)}\left[b_B||\bm{u}^{rc}(\tau)+b_Bb_T\right]d\tau\\
    &\leq||\bm{x}(0)||e^{(c_f-\lambda)t}+\int^t_0e^{(c_f-\lambda)(t-\tau)}b_B||\bm{u}^{rc}(\tau)||d\tau+\int^t_0e^{(c_f-\lambda)(t-\tau)}b_Bb_Td\tau 
    \label{eq:x_int}
\end{align}
Furthermore, taking the $\lambda$ norm in both terms of Eq.~\ref{eq:x_int}
\begin{align}
    ||\bm{x}(t)||_{\lambda}&\leq||\bm{x}(0)||+\frac{b_B}{\lambda-c_f}(1-e^{(c_f-\lambda)T'})||\bm{u}^{rc}(t)||_{\lambda}+\frac{b_Bb_T}{\lambda-c_f}(1-e^{(c_f-\lambda)T'})\\
    &\leq||\bm{x}(0)||+\frac{b_B}{\lambda-c_f}(1-e^{(c_f-\lambda)T'})||\bm{u}^{rc}(t)||_{\lambda}+\epsilon'
\end{align}
where 
\begin{equation}
    \epsilon'=\frac{b_Bb_T}{\lambda-c_f}(1-e^{(c_f-\lambda)T'})
\end{equation}
So, 
\begin{equation}
    \lim_{t\rightarrow\infty}\sup||\bm{x}(t)||\leq||\bm{x}(0)||+\frac{b_B}{\lambda-c_f}(1-e^{(c_f-\lambda)T'})\frac{1}{1-\bar{\rho}}\epsilon+\epsilon'
    \label{eq:lim_x}
\end{equation}
Then it can be shown from Eqs.~\ref{eq:eps} and~\ref{eq:lim_x} that the attitude tracking error bounds depend on the initial tracking error, the disturbance, and the time shift $\Delta$. The anticipatory scheme requires $\Delta > 0$, but it can be small enough to designate the bounds if necessary.
